# Supplementary material for: Towards Trustworthy Dataset Distillation
Source: arXiv:2307.09165 source file (2024-08-11)

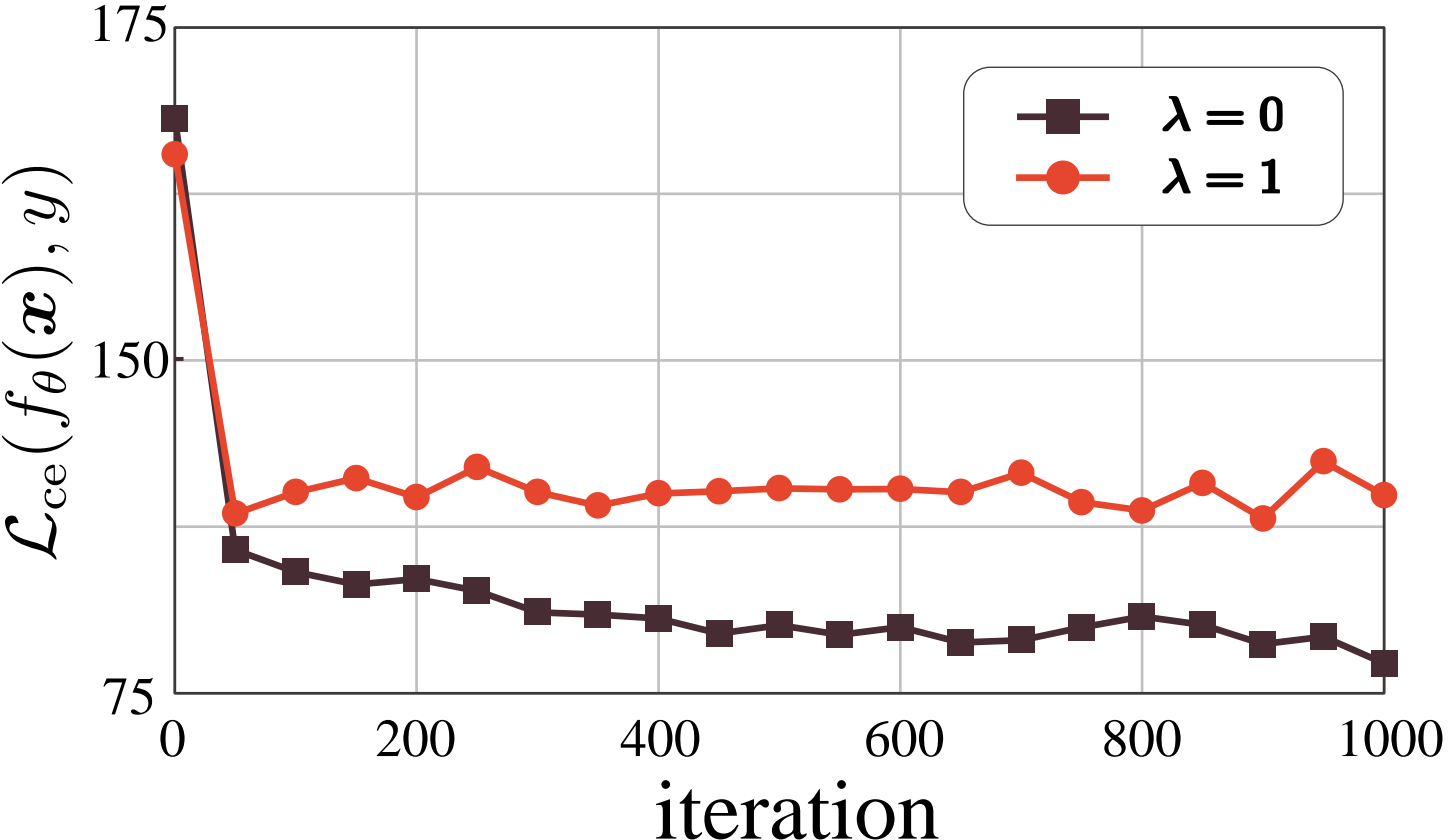

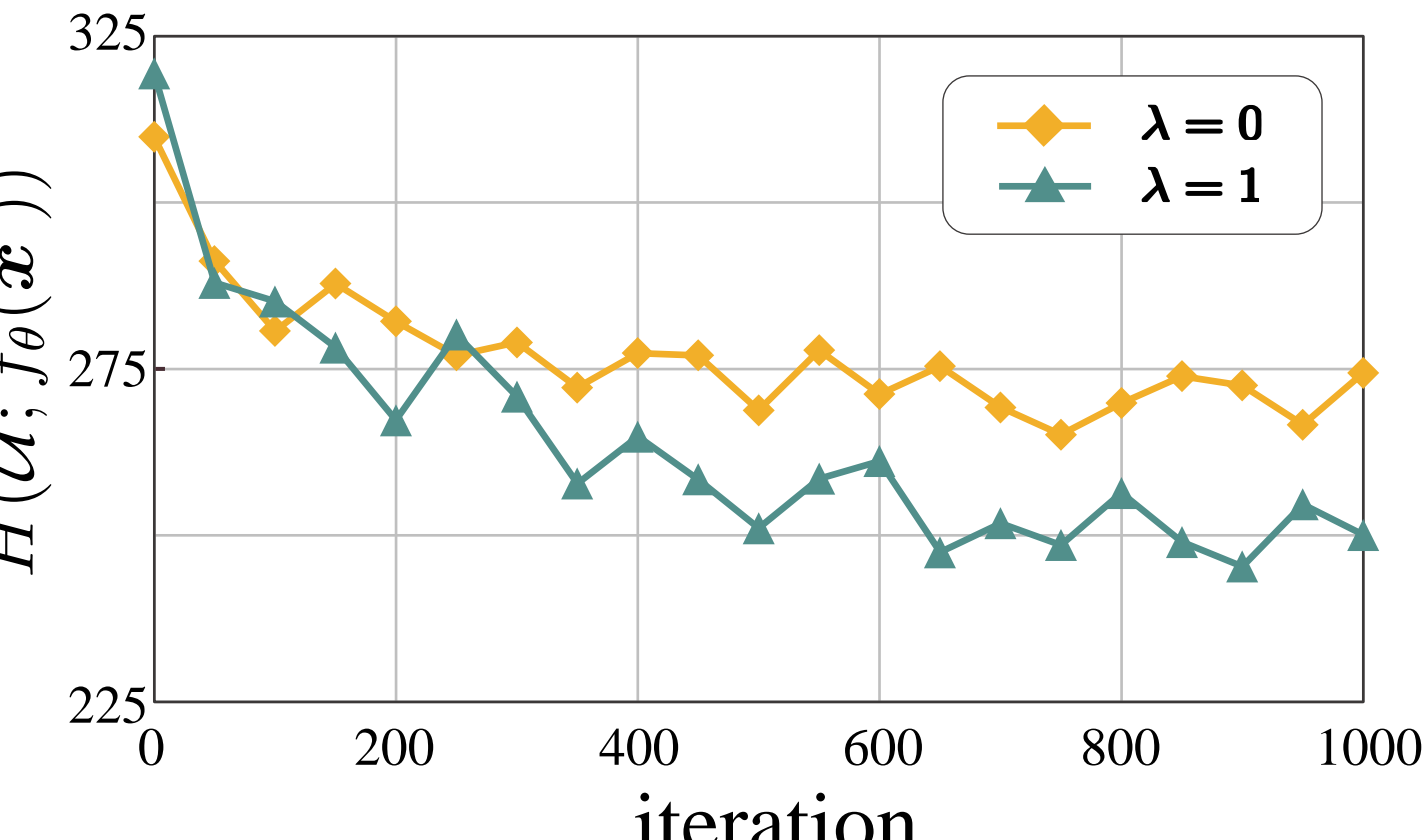

Supplement: Supplementary file 1 [file ce-loss-iter.pdf]
